# Supplementary material for: Breaking the Familiarity Bias: Employing Virtual Reality Environments to Enhance Team Formation and Inclusion
Source: arXiv:2502.09912 source file (2025-02-14)
Supplement: Supplementary file 1 [file Resumes.pdf]

## **University President Selection Meeting**

### **Job Title:**

President, University Satellite Campus

### **Job Summary:**

The University is seeking a dynamic and visionary leader to serve as the President of our newly established campus. The President is responsible for providing strategic direction, fostering academic excellence, and creating a vibrant and inclusive campus community. This is a unique opportunity to shape the identity and growth of a satellite campus while upholding the esteemed traditions and values of the University.

### **Preferred Qualifications:**

- *A terminal degree in a relevant field*
- *Significant leadership experience in higher education administration*
- *Proven track record of strategic planning and execution*
- *Strong commitment to academic excellence and fostering a supportive campus community*
- *Excellent interpersonal and communication skills*
- *Demonstrated ability in fundraising and resource development*

***Attached is information on the 3 candidates for consideration.***

## Candidates for President of New Campus

| <u>Candidate:</u> | <u>CV Highlights:</u>                                                                                                                        | <u>Additional information from interviews:</u>                                                                                                                                                                                                                                                                                                                                                                                                                                                                            |
|-------------------|----------------------------------------------------------------------------------------------------------------------------------------------|---------------------------------------------------------------------------------------------------------------------------------------------------------------------------------------------------------------------------------------------------------------------------------------------------------------------------------------------------------------------------------------------------------------------------------------------------------------------------------------------------------------------------|
| <b>Stevens</b>    | <ul style="list-style-type: none"><li>• Provost</li><li>• Former Dean</li><li>• Plans for money/donations</li><li>• Full professor</li></ul> | Stevens, a candidate of diverse talents, left a fundraising role without significant funds raised and was not responsible for donations. However, their national recognition as a researcher and endorsement by business leaders underscores their expertise beyond fundraising. Stevens emphasizes collaboration, possesses strong oratory skills, and is engaged in consulting work. Teaching a module and having a spouse who teaches Spanish highlight their commitment to education and a multicultural environment. |

---

| <u>Candidate:</u> | <u>CV Highlights:</u>                                                                                                                                      | <u>Additional information from interviews:</u>                                                                                                                                                                                                                                                                                                                                                                  |
|-------------------|------------------------------------------------------------------------------------------------------------------------------------------------------------|-----------------------------------------------------------------------------------------------------------------------------------------------------------------------------------------------------------------------------------------------------------------------------------------------------------------------------------------------------------------------------------------------------------------|
| <b>Roberts</b>    | <ul style="list-style-type: none"><li>• Political leader</li><li>• Former Dean at 2 universities</li><li>• Raised money</li><li>• Full professor</li></ul> | Roberts is perceived as aloof and has been out of higher education for four years, lacking campus and student life experience. Accusations of changing positions have been noted. Roberts is actively involved in volunteer work, possesses influential contacts, and is recognized as an excellent teacher. Past achievements include securing a grant. Additionally, Roberts maintains an apartment in Spain. |

---

| <u>Candidate:</u> | <u>CV Highlights:</u>                                                                                                                                     | <u>Additional information from interviews:</u>                                                                                                                                                                                                                                                                                                  |
|-------------------|-----------------------------------------------------------------------------------------------------------------------------------------------------------|-------------------------------------------------------------------------------------------------------------------------------------------------------------------------------------------------------------------------------------------------------------------------------------------------------------------------------------------------|
| <b>Jones</b>      | <ul style="list-style-type: none"><li>• Senior manager</li><li>• Steering Committee</li><li>• Argued in High Court</li><li>• Visiting Professor</li></ul> | Jones is noted for having a temper and a high turnover, portraying an abrasive leadership style. Jones exhibits a pleasant personality, is a strategic thinker, and serves as an active trustee. As a teacher, students appreciate them. Living locally, Jones has a grown-up child and enjoys mystery novels and biographies in their leisure. |

## Candidates for President of New Campus

| <u>Candidate:</u> | <u>CV Highlights:</u>                                                                                                                        | <u>Additional information from interviews:</u>                                                                                                                                                                                                                                                                                                                                                                                                    |
|-------------------|----------------------------------------------------------------------------------------------------------------------------------------------|---------------------------------------------------------------------------------------------------------------------------------------------------------------------------------------------------------------------------------------------------------------------------------------------------------------------------------------------------------------------------------------------------------------------------------------------------|
| <b>Stevens</b>    | <ul style="list-style-type: none"><li>• Provost</li><li>• Former Dean</li><li>• Plans for money/donations</li><li>• Full professor</li></ul> | Stevens exhibits a tendency to discourage innovation and isn't responsible for donations. Despite this, Stevens is nationally recognized as a researcher, earning praise from business leaders. Stevens demonstrates strong oratory skills and emphasizes collaboration. Personally, family is a significant aspect, with a spouse and three kids, and the presence of family nearby. Outside of professional pursuits, Stevens enjoys gardening. |

---

| <u>Candidate:</u> | <u>CV Highlights:</u>                                                                                                                                      | <u>Additional information from interviews:</u>                                                                                                                                                                                                                                                                                                                                                                                                    |
|-------------------|------------------------------------------------------------------------------------------------------------------------------------------------------------|---------------------------------------------------------------------------------------------------------------------------------------------------------------------------------------------------------------------------------------------------------------------------------------------------------------------------------------------------------------------------------------------------------------------------------------------------|
| <b>Roberts</b>    | <ul style="list-style-type: none"><li>• Political leader</li><li>• Former Dean at 2 universities</li><li>• Raised money</li><li>• Full professor</li></ul> | Roberts is perceived as aloof and has been out of higher education for four years, lacking campus and student life experience. Roberts is actively involved in volunteer work, showcasing a commitment to community engagement. Known as a thoughtful leader and listener, Roberts excels in collaborative decision-making. Recognized as an excellent teacher, Roberts has a track record of securing grants and enjoys playing golf and tennis. |

---

| <u>Candidate:</u> | <u>CV Highlights:</u>                                                                                                                                     | <u>Additional information from interviews:</u>                                                                                                                                                                                                                                                                                    |
|-------------------|-----------------------------------------------------------------------------------------------------------------------------------------------------------|-----------------------------------------------------------------------------------------------------------------------------------------------------------------------------------------------------------------------------------------------------------------------------------------------------------------------------------|
| <b>Jones</b>      | <ul style="list-style-type: none"><li>• Senior manager</li><li>• Steering Committee</li><li>• Argued in High Court</li><li>• Visiting Professor</li></ul> | Jones is noted for having a temper and a decreased success rate in court. Jones has a pleasant personality and strategic thinking. An active trustee and well-liked teacher, Jones leads a household with two cats and two dogs. Their spouse is a physician, and in leisure, Jones enjoys reading mystery novels and biographies |

## Candidates for President of New Campus

| <u>Candidate:</u> | <u>CV Highlights:</u>                                                                                                                        | <u>Additional information from interviews:</u>                                                                                                                                                                                                                                                                                                               |
|-------------------|----------------------------------------------------------------------------------------------------------------------------------------------|--------------------------------------------------------------------------------------------------------------------------------------------------------------------------------------------------------------------------------------------------------------------------------------------------------------------------------------------------------------|
| <b>Stevens</b>    | <ul style="list-style-type: none"><li>• Provost</li><li>• Former Dean</li><li>• Plans for money/donations</li><li>• Full professor</li></ul> | Stevens has been observed drinking heavily and left a fundraiser without raising funds. Despite this, Stevens is nationally recognized as a researcher, endorsed by business leaders. Known for emphasizing collaboration and possessing strong oratory skills, Stevens also enjoys a range of activities, including sports, biking, running, and gardening. |

---

| <u>Candidate:</u> | <u>CV Highlights:</u>                                                                                                                                      | <u>Additional information from interviews:</u>                                                                                                                                                                                                                                                                                                                                               |
|-------------------|------------------------------------------------------------------------------------------------------------------------------------------------------------|----------------------------------------------------------------------------------------------------------------------------------------------------------------------------------------------------------------------------------------------------------------------------------------------------------------------------------------------------------------------------------------------|
| <b>Roberts</b>    | <ul style="list-style-type: none"><li>• Political leader</li><li>• Former Dean at 2 universities</li><li>• Raised money</li><li>• Full professor</li></ul> | Roberts is seen as aloof with four years out of higher education, lacking campus and student life experience. However, Roberts excels as an excellent teacher, fostering increased faculty research productivity and diversity. Notably, Roberts has secured a grant. Despite personal challenges like divorce, Roberts has remarried, has two children, and follows a vegetarian lifestyle. |

---

| <u>Candidate:</u> | <u>CV Highlights:</u>                                                                                                                                     | <u>Additional information from interviews:</u>                                                                                                                                                                                                                                                                                              |
|-------------------|-----------------------------------------------------------------------------------------------------------------------------------------------------------|---------------------------------------------------------------------------------------------------------------------------------------------------------------------------------------------------------------------------------------------------------------------------------------------------------------------------------------------|
| <b>Jones</b>      | <ul style="list-style-type: none"><li>• Senior manager</li><li>• Steering Committee</li><li>• Argued in High Court</li><li>• Visiting Professor</li></ul> | Jones experiences tension with the provost and is associated with high turnover due to an abrasive leadership style. Jones maintains a pleasant personality and is recognized as a strategic thinker. As an active trustee and well-liked teacher, Jones finds enjoyment in playing bridge, traveling, and indulging in a love for cooking. |
